# Supplementary material for: A Structured Framework for Predicting Sustainable Aviation Fuel Properties using Liquid-Phase FTIR and Machine Learning
Source: arXiv:2408.01530 ancillary file (2024-08-02)
Supplement: Supplementary file 1 [file SI.pdf]

## Supplemental Information for
## A Structured Framework for Predicting Sustainable Aviation Fuel Properties using Liquid-Phase FTIR and Machine Learning

*Ana E. Comesana, Sharon S. Chen, Kyle E. Niemeyer, and Vi H. Rapp*

### S-1. FTIR-Attenuated Total Reflectance (ATR) Fuel Preparation and Measurements

A summary of the equipment and procedures for preparing fuel samples and measuring liquid-phase FTIR-ATR spectra are provided in the following subsections.

#### *S-1.1. Fuel samples and equipment preparation*

To prepare the fuel samples, we used the following equipment and supplies:

- Chromatography vials (4mL) with septum caps for storage of sample
  - Amber glass is preferred clear glass can be used if covered with foil to limit light exposure
  - Septum must be PTFE or other material compatible with samples
- Vial rack for storage and transportation
- Vial labels
- Vial clamp or holder
- Methanol, residue analysis grade
- Borosilicate glass Pasteur pipets and pipet bulbs
- Kimwipes
- Beaker for excess chemicals
- 1 or more Syringe (1 mL volume) with stainless steel beveled needle tip of gauge 22-26
- 1 or more Syringe (0.1 mL volume) with stainless steel beveled needle tip of gauge 22-26

Prior to mixing fuels, we detergent-washed and air-dried all glassware. We then prepared suitable working containers for each neat fuel by rinsing the container three times with the fuel it will house and applying appropriate labels. Next, we transferred the desired volume of each neat sample from its primary container to the working container using clean glass Pasteur pipets with a pipet bulb. New pipets were used for each fuel. The intent of this process is to protect the primary (original) containers of neat fuel from accidental

contamination that might occur during the mixing process. We refilled the working containers as needed and replaced them if they became contaminated. Pre-cleaned chromatography vials were used as-received. Next, we solvent-wash syringes before use to prevent contamination using the following procedure:

- Prepare a wash bottle filled with methanol
- Prepare 2 small Erlenmeyer flasks (with caps/plugs or foil covers) filled with methanol, and a clean empty glass beaker. Label one flask "MeOH 1," the other flask "MeOH 2.," and the clean beaker "Excess."
- Hold syringe above the "Excess" beaker and use the wash bottle to rinse the outside of syringe (barrel included) with methanol, then wipe dry with a Kimwipe. Do this twice.
- Uncap "MeOH 1." Use the syringe to draw a full volume of methanol from MeOH1, then dispense to the "Excess" beaker. Do this a minimum of 3 times. When finished, cap "MeOH 1."
- Uncap "MeOH 2." Use the syringe to draw a full volume of methanol from "MeOH 2," then dispense to the "Excess" beaker. Do this a minimum of 3 times. When finished, cap "MeOH 2."
- Use a Kimwipe to dry the external surfaces of the syringe and needle. The syringe is now solvent-washed. Set aside on a clean Kimwipe in the fume hood until use.

Syringes were solvent-washed at the start of a mixing session, the end of a mixing session, and before using different fuels. Next, we conducted a dead volume flush with the fuel sample to prevent contamination. This ensured the small volume of liquid that remains in the syringe needle even after the plunger is fully depressed does not contaminate the fuel mixture. The flushing procedure is as follows:

- Using a solvent-washed syringe , slowly draw a full volume of the fuel sample from the working container (air bubbles in the barrel can be ignored as this is not a measurement). Then, fully dispense the sample into the "Excess" beaker.
- Use a Kimwipe to wipe dry the outside of the syringe needle.
- Repeat this process (i.e. draw and then dispense a full volume of the fuel to "Excess") a minimum of 3 times.
- Note: To prevent contamination, do not push down on the plunger until the syringe is fully removed from the fuel sample working container. If the working container becomes contaminated, discard it and prepare a new fuel sample working container.

- Note: To minimize waste of the fuel sample, additional syringes could be used and dedicated to a specific fuel sample or fuel mixtures can be prepared in an order that reduces the number solvent-washes for a given syringe. Smaller flush volumes could also be used as long as the volume exceeds the draw volume of the fuel, or testing validates that the level of possible contamination is undetectable by the FTIR measurement.

After cleaning syringes and preparing neat fuels, we prepared the fuel mixtures. Fuel mixtures were not prepared more than 24 hours before the FTIR measurement. This minimized any errors that might arise from sample loss during storage. Prior to mixing, we calculated the quantities of each fuel sample needed for each mixture. Next, we selected syringes that were appropriately sized for measuring the required quantities of the neat fuel samples to ensure the septum would not be punctured more than 3 times in total. For example, Table S1 shows the accuracy and manufacturer-specified minimum draw volumes of our two syringes (1 mL and 0.1 mL). We used the 0.1 mL syringe for draw volumes less than 0.1 mL, and the 1 mL syringe for draw volumes 0.1 mL and larger. This arrangement maximizes our draw volume accuracy while limiting septum punctures to 3 or fewer.

Table S1: Capacity and accuracy of syringes used for fuel mixing

| Syringe Volume | Accuracy | Minimum Volume |
|---|---|---|
| 1 mL | 0.01 mL | 0.1 mL |
| 0.1 mL | 0.001 mL | 0.01 mL |

After solvent-washing and dead-flushing the syringes with the appropriate fuel samples, we then mixed the fuels using the following procedure:

- Prepare or refill working containers for each neat fuel sample that will be used in the mixing session. There should be enough fuel in each container to accommodate the quantity that will be used during the session.

- Prepare one clean 4 mL vial and septum cap. Label the vial with the mixture code or name and preparation date. Secure the labeled vial in the vial clamp.

- Uncap the working container of Fuel 1 and insert the needle tip of the prepared syringe (solvent-washed and dead-flushed) into the liquid.

- Hold the syringe so that the tip does not touch the walls of the container and is well below the liquid surface.

- Slowly pull up on the plunger to begin filling the syringe with fuel.

- Draw out a volume of fuel that is larger than the target draw volume. At minimum, the overdraw must be at minimum the volume of any air bubbles within the syringe barrel plus the dead volume of the syringe.
- Remove the syringe from the working container, then cap the working container.
- To remove undesirable air bubbles within the syringe barrel:
  - Invert the syringe so that the needle tip points directly upwards. The bubbles should float upwards and coalesce at the inlet of the syringe barrel. If they do not, gently tap on the syringe barrel so that the vibrations dislodge any bubbles stuck to the interior surfaces of the syringe.
  - Wrap a clean Kimwipe loosely around the needle tip.
  - With the syringe still inverted, slowly push in the plunger until the air bubble at the syringe inlet is completely evacuated from the barrel.
  - Continue pushing in the plunger until the plunger tip is aligned with the line marking of the target volume. Note: the Kimwipe will absorb the small amount of fuel expelled during this process and ensure the dead space in the syringe is filled with liquid instead of air.
- Gently dry off the needle tip with a Kimwipe, taking care to neither wick liquid from inside the syringe tip, nor plug the tip with stray lint or fibers. The syringe is now ready to dispense Fuel 1 to the labeled 4 mL vial.
- Unscrew the septum cap of the labeled mixture vial halfway. It should be loose enough to allow the passage of air, but not so loose that it will fall off during handling.
- While gripping the syringe by the top of the barrel (to avoid accidentally depressing the plunger), align the syringe needle above the loosely-capped vial so it is in-line with the center of vial body. If the septum has already been pierced, aim for the same location. Remember that a given septum should not be punctured more than 3 times.
- Gently push the syringe downward so the needle tip gently pierces through the center of the septum. Continue pushing the barrel of the syringe downward until the needle tip is inserted halfway into the empty airspace of the vial. Take care not to misalign the syringe body and break the needle tip.
- Depress the plunger slowly to dispense the drawn volume of Fuel 1 to the empty vial. During this process, keep the needle tip continually above the liquid level. After the plunger is fully depressed, any droplets still clinging to the needle tip can be dislodged through gentle tapping on the syringe barrel.

- Slowly remove the syringe needle from the septum cap by pulling up on the syringe barrel.
- Wipe dry the entire length of the syringe needle tip with a clean Kimwipe wetted with a small amount of methanol. If the next draw on the syringe will use the same fuel, set it aside on a clean Kimwipe to dry (approximately 1 minute) until the next use. If the next draw will be of a different fuel, the syringe must be solvent-washed as described in a previous section.
- Tighten the septum cap of the mixture vial until snug. Do not overtighten as this will damage the septum.
- Repeat steps above to add the target volume of Fuel 2 to the labeled 4 mL mixture vial.
- After adding all fuels and ensuring the septum cap is installed snugly on the vial, remove the vial from the vial clamp.
- Mix the contents by gently shaking the vial back and forth for no less than 30 seconds.
- Visually inspect the vial to ensure that no liquid has been lost from the vial
- If necessary, wrap vial cap with container seal and wrap clear vials in aluminum foil to prevent sample loss and protect contents from light exposure, respectively.
- Store prepared mixture vials upright in a vial rack and place in a flammables cabinet until FTIR measurements can be made (maximum 24 hours).
- At the end of a mixing session, solvent-wash all syringes and tightly cap all working containers. Return the working containers to the flammables cabinet. Dispense contents of the "Excess" beaker to hazardous waste collection.

*S-1.2. FTIR-ATR Measurements*

To collect FTIR-ATR spectra measurements of the liquid fuel samples, we used the following equipment and supplies:

- Thermo Scientific Nicolet iS50 FTIR Spectrometer (w/ OMNIC software)
- Thermo Scientific Smart iTR ATR sampling accessory (diamond crystal w/ ZnSe lens)
- Isopropyl Alcohol
- Kimwipes or cotton balls/swabs
- Borosilicate glass Pasteur pipets & pipet bulbs

- Stainless steel tweezers or forceps (for material handling)
- Viton square-profile O-rings (for sample containment on ATR)
- 316 stainless steel tags (for sample containment on ATR)

Prior to collecting measurements, we install the Smart iTR ATR sampling accessory in iS50 main compartment following the manufacturer's instructions. We initiate the OMNIC software and confirm that it recognizes the Smart iTR accessory and then verify and adjust experiment settings to match the following:

- Change the default ATR experimental settings from "Default iS50 ATR.exp" to "Smart iTR diamond iTR" using the Experiment drop-down menu.
- Update the appropriate settings on "iTR Diamond.exp" to match the following. Any settings not specified below can be left as the default. The Experiment Setting window is reachable via the "Expt Set" button.
  - Collect Tab:
    - Number of scans: 64
    - Resolution: 2 cm-1
    - Final format: Absorbance
    - Correction: None
    - Check the Preview data collection checkbox (optional, but recommended)
    - Background collection frequency can be set to before every scan, or by time interval. I prefer to manually initiate background scans before every measurement, so I do not bother changing the time interval from the default of 120 min
  - Bench tab:
    - Sample compartment: Main
    - Detector: DTGS KBr
    - Beamsplitter: KBr
    - Source: IR
    - Accessory: Smart iTR
    - Window: Diamond (default). Although our version of the accessory has a laminated diamond crystal, Thermo Fisher Scientific Tech Support assured me that this parameter only changes the default wavelength ranges and does not apply any corrections to the scan. I've opted to keep the default.

- Wavelength range: 4000 cm-1 to 650 cm-1
- Gain: 1.0
- Optical velocity: 0.4747
- Aperture: 80 (default)
- Attenuation: None

Next, we waited 1 hour before beginning measurements to minimize background signals of CO2 and water vapor. While waiting, we cleaned the ATR crystal plate twice with isopropyl alcohol and cleaned Kimwipes and prepared our tools and samples. When cleaning the crystal plate the first time, we used a wash bottle to dispense a small amount of isopropyl alcohol directly onto the crystal plate and then gently patted it dry with a Kimwipe. For the second cleaning, we wetted a Kimwipe with isopropyl alcohol patted it onto the crystal plate, and pat-dried the crystal with a new Kimwipe. Note, we never use wiping motions on the crystal as it can cause damage. We also cleaned the pressure tower tip with isopropyl alcohol. After the Smart iTR has warmed up in the main compartment for 1 hour, we align instrument optics then began the measurement session using the following procedures:

1. Using clean tweezers/forceps, place a Viton O-ring onto the crystal plate such that the crystal is centered in the O-ring hole. Be careful not to contact the crystal with either the tweezers/forceps or the O-ring. Push down on the O-ring to ensure good contact with the plate surface.
2. Initiate a background scan: Collect > Collect Background, or by pressing the "Col Bkg" button.
3. While the background scan is being collected, prepare the sample vial by removing the foil and any sealing material and then gently shaking the vial contents for  10 seconds. Secure the vial in the vial clamp. Retrieve a clean pipet and pipet bulb.
4. Inspect background scan to identify any abnormalities such as unexpected peaks, premature wavelength cutoffs, etc. If none, proceed to the sample scan.
5. Load the liquid fuel sample onto the ATR crystal within 8-seconds to minimize evaporation by doing the following:

    - Unscrew the cap from the sample vial and insert the tip of the clean glass pipet into the vial so that it is well below the liquid surface, but not touching the vial walls or bottom. Gently draw up a small amount of the fuel sample(  3-5 droplets of sample or 30-50 mL).
    - Bring the loaded pipet over to the crystal and gently deposit 3-5 drops into the center of the O-ring. Fill the sample well such that it is roughly 1/2 to 3/4 full to minimize effects of evaporation. Do not overfill.

- Using tweezers/forceps, cover the O-ring with a clean stainless steel tag
- Then swing the pressure tip forward (clockwise rotation) and twist the pressure tower knob until the tip touches the tag. Keep twisting the knob clockwise until you hear it click (it will slip once a given pressure is achieved).

6. Click “Collect” to initiate the sample scan.
7. Screw the cap back on to the sample and place it back into the sample tray.
8. After scan is complete, disengage the pressure clamp by twisting the tower knob counterclockwise. Swing the pressure tip to the side so that it is out of the way.
9. Use the tweezers/forceps designated for contaminated materials to remove the SS tag and O-ring off the crystal plate and place them immediately into a sealed hazardous waste bag.
10. Use a dry Kimwipe to pat dry the liquid fuel sample pooled on top of the crystal plate, absorbing as much liquid as possible. Discard this used Kimwipe to the hazardous waste bag.
11. Clean the crystal using the two-step isopropyl alcohol cleaning procedure conducted previously.
12. Confirm all fuel traces have been cleaned by initiating a sample scan (with no sample) with the “preview data collection” mode active. Verify that the signal looks like baseline noise with no unexpected peaks.

The steps above were repeated for all fuel mixture samples. Figure S1 shows the experimental setup with the O-ring and stainless steel tag. Additionally, the first measurement and last measurement of every session was a reference sample (i.e., Jet A) to validate repeatability and accuracy of measurements between sessions. To improve this method, we recommend future work investigate the performance of other septum materials, and explore alternative methods of priming the syringe needles when drawing fuel sample.

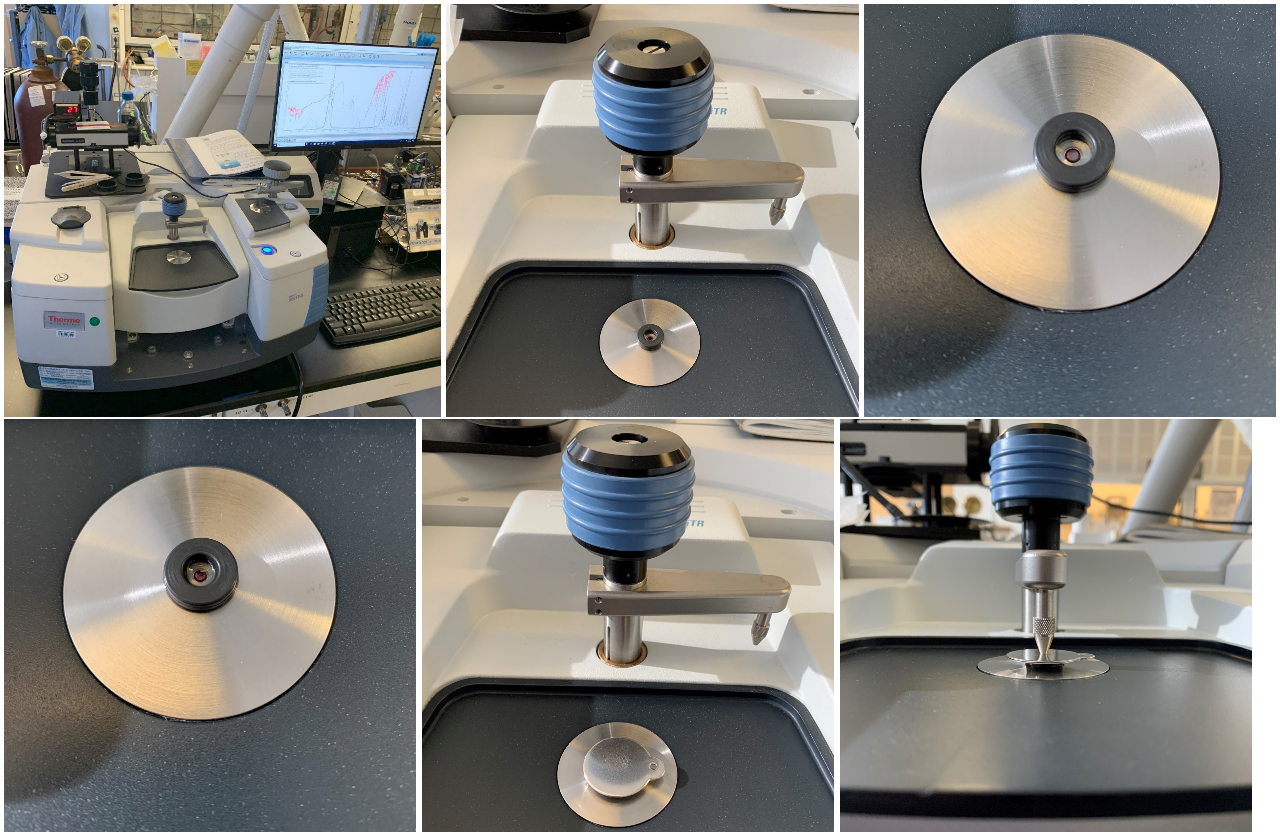

Figure S1: Experimental procedure for measuring liquid FTIR-ATR spectra of fuel samples with (a) FTIR instrument with ATR accessory, (b) ATR accessory with the Viton square-profile O-ring for sample containment, (c) O-rings placement around the ATR crystal, (d) O-ring with a fuel sample inside, (e) stainless steel tag placed on top of the O-ring, and (f) pressure tip secured on top of the stainless steel tag.

## S-2. Model Metrics

Model performance metrics in the train, validation, and test sets is shown in Table ]S2.

Table S2: Performance for the five property prediction models on training data and all data. Density is measured at 15 °C and viscosity is measured at −20 °C.

| | Final boiling point | Flash point | Freezing point | Density | Kinematic Viscosity |
|---|---|---|---|---|---|
| Train MAE | 13.8 K | 7.6 K | 8.1 K | 12.2 $\frac{kg}{m^3}$ | 0.33 $\frac{mm^2}{s}$ |
| Overall MAE | 15.6 K | 8.6 K | 9.4 K | 16 $\frac{kg}{m^3}$ | 0.42 $\frac{mm^2}{s}$ |
| Train RMSE | 19.2 K | 11.2 K | 11.8 K | 17.8 $\frac{kg}{m^3}$ | 0.44 $\frac{mm^2}{s}$ |
| Overall RMSE | 22.9 K | 13.8 K | 14.4 K | 26.9 $\frac{kg}{m^3}$ | 0.64 $\frac{mm^2}{s}$ |
| Train MAPE | 3.5% | 2.7% | 5% | 1.7% | 21.7% |
| Overall MAPE | 4.1% | 3% | 5.7% | 2.1% | 34.9% |

## S-3. All compounds used

Table S4 shows a list of all neat molecules, aviation fuels, and blends used to train the property prediction models.

Table S3: List of all compounds used (part 1). Calculated values were determined using linear-by-volume

| Name | Formula | CAS | Final boiling point | Final boiling point source | Flash point | Flash point source | Freezing point | Freezing point source | Density ($kg/m^3$) | Density source | Kinematic viscosity ($mm^2/s$) | Kinematic viscosity source |
|---|---|---|---|---|---|---|---|---|---|---|---|---|
| 1,2,3,4-tetrahydronaphthalene | C10H12 | 119-64-2 | 480.7 | [1] | 352.2 | [1] | 238.7 | [1] | 970.2 | [2] | 0.952 | [2] |
| 1,2,3,4-tetramethylbenzene | C10H14 | 488-23-3 | 478.1 | [3] | | | 266.9 | [3] | 903.9 | [2] | | |
| 1,2,3-trimethylbenzene | C9H12 | 526-73-8 | 448.1 | [1] | 318.8 | [1] | 247.8 | [1] | 892.2 | [2] | | |
| 1,2,4-trimethylbenzene | C9H12 | 95-63-6 | 442.1 | [1] | 317.3 | [1] | 229.3 | [1] | 875.8 | [2] | | |
| 1,3,5-trimethylbenzene | C9H12 | 108-67-8 | 438.0 | [1] | 323.1 | [1] | 228.3 | [1] | 857.4 | [2] | | |
| 1-hexene | C6H12 | 592-41-6 | 336.5 | [1] | 247.0 | [1] | 133.4 | [1] | 697.9 | [2] | 0.58 | [2] |
| 1-methylnaphthalene | C11H10 | 90-12-0 | 516.1 | [1] | 355.1 | [1] | 251.2 | [1] | | | | |
| 1-pentene | C5H10 | 109-67-1 | 303.1 | [1] | | | 108.0 | [1] | 640.8 | [2] | 0.44 | [2] |
| 2,3-dimethylpentane | C7H16 | 565-59-3 | 362.9 | [2] | | | | | 695.1 | [2] | | |
| 2,4-dimethylhexane | C8H18 | 589-43-5 | 382.6 | [4] | | | | | 701.8 | [2] | | |
| 2,4-dimethylpentane | C7H16 | 108-08-7 | 353.6 | [1] | | | 153.2 | [3], [1] | 672.5 | [2] | | |
| 2,5-dimethylhexane | C8H18 | 592-13-2 | 382.2 | [1] | | | 182.2 | [5],[1] | 693.8 | [2] | | |
| 2-butanol | C4H10O | 78-92-2 | 372.7 | [1], [4] | 298.8 | [1], [4], [6] | 158.4 | [1], [5] | 807.6 | [2] | | |
| 2-ethyl-p-xylene | C10H14 | 1758-88-9 | 460.1 | [7] | | | 219.4 | [3] | 877.2 | [2] | | |
| 2-methyl-1-butene | C5H10 | 563-46-2 | 304.4 | [1] | | | 135.7 | [1] | 648.4 | [2] | | |
| 2-methyl-2-butene | C5H10 | 513-35-9 | 311.4 | [1] | 255.3 | [1] | 139.5 | [1], [5] | 658.0 | [2] | | |
| 2-methylbutane | C5H12 | 78-78-4 | 301.0 | [1] | 216.5 | [1], [6] | 113.3 | [1], [5] | 620.1 | [2] | 0.535 | [2] |
| 2-methylhexane | C7H16 | 591-76-4 | 363.1 | [1], [4] | 255.2 | [4], [6] | 155.2 | [1], [5] | 683.2 | [2] | | |
| 2-methylpentane | C6H14 | 107-83-5 | 332.6 | [1] | 247.2 | [1] | 119.7 | [1], [5] | 655.0 | [2] | | |
| 2-pentene | C5H10 | 109-68-2 | 309.9 | [1] | | | 127.3 | [3] | | | | |
| 2-propyltoluene | C10H14 | 1074-17-5 | 458.1 | [1] | | | 212.8 | [3] | 874.3 | [2] | | |
| 3-ethyl-2-methylpentane | C8H18 | 609-26-7 | | | | | | | 719.3 | [2] | | |
| 3-methylhexane | C7H16 | 589-34-4 | 364.1 | [1], [4] | | | 154.2 | [1], [5] | | | | |
| 3-methylpentane | C6H14 | 96-14-0 | 336.4 | [1] | 266.6 | [1] | 110.2 | [1] | 664.3 | [2] | 0.6635 | [2] |
| 4-ethyl-m-xylene | C10H14 | 874-41-9 | 461.6 | [2] | | | 210.2 | [3] | 867.2 | [2] | | |
| anisol | C7H8O | 100-66-3 | 427.7 | [1] | 325.0 | [1] | 235.8 | [1] | | | | |
| butylcyclohexane | C10H12 | 1678-93-9 | 454.1 | [1], [4] | | | 198.4 | [1], [4] | 799.2 | [2] | 3.55 | [2] |
| cumene | C9H12 | 98-82-8 | 425.4 | [1], [4] | 309.6 | [1] | 177.0 | [1] | 897.3 | [2] | 1.567 | [2] |
| cyclohexane | C6H12 | 110-82-7 | 353.9 | [1], [4] | 254.3 | [1], [4], [6] | 279.8 | [1], [5] | 778.5 | [2] | | |
| cyclopentane | C5H10 | 287-91-3 | 322.4 | [1] | 236.0 | [1], [6] | 179.3 | [1], [5] | 745.7 | [2] | 0.92 | [2] |
| diisobutylene | C8H16 | 107-39-1 | 374.4 | [1] | 268.1 | [1] | 179.8 | [1] | 712.9 | [2] | | |
| 20% heptane, 70% isooctane, 10% ethanol | | | 370.1 | Calculated | 276.9 | Calculated | 168.6 | Calculated | 697.8 | Calculated | | |
| 20% heptane, 79% isooctane, 1% ethanol | | | 371.9 | Calculated | 276.2 | Calculated | 169.2 | Calculated | 688.8 | Calculated | | |
| 20% heptane, 75% isooctane, 5% ethanol | | | 371.1 | Calculated | 276.5 | Calculated | 168.9 | Calculated | 692.8 | Calculated | | |
| 20% heptane, 70% isooctane, 10% toluene | | | | | | | | | | | | |
| 30% heptane, 60% isooctane, 10% ethanol | | | 370.0 | Calculated | 276.1 | Calculated | 170.2 | Calculated | 696.7 | Calculated | | |
| 30% heptane, 69% isooctane, 1% ethanol | | | 371.9 | Calculated | 275.4 | Calculated | 170.8 | Calculated | 687.8 | Calculated | | |
| 30% heptane, 65% isooctane, 5% ethanol | | | 371.0 | Calculated | 275.7 | Calculated | 170.6 | Calculated | 691.8 | Calculated | | |
| 45% heptane, 55% ethanol | | | | | | | | | | | | |
| 55% heptane, 45% ethanol | | | | | | | | | | | | |
| 90% heptane, 10% toluene | | | | | | | | | | | | |
| heptane | C7H16 | 142-82-5 | 371.6 | [1] | 269.8 | [1], [6] | 182.6 | [1], [5] | 679.8 | [2] | 0.9639 | [2] |
| isooctane | C8H18 | 540-84-1 | 372.3 | [1] | 277.6 | [1] | 165.9 | [1], [5] | 689.9 | [2] | 1.1938 | [2] |
| methylcyclohexane | C7H14 | 108-87-2 | 374.1 | [1], [4] | 268.8 | [1], [6] | 146.6 | [1], [5] | 767.7 | [2] | 1.75 | [2] |

Table S4: List of all compounds used (part 2). Calculated values were determined using linear-by-volume

| Name | Formula | CAS | Final boiling point | Final boiling point source | Flash point | Flash point source | Freezing point | Freezing point source | Density ($kg/m^3$) | Density source | Kinematic viscosity ($mm^2/s$) | Kinematic viscosity source |
|---|---|---|---|---|---|---|---|---|---|---|---|---|
| n-pentane | C5H12 | 109-66-0 | 309.3 | [1], [4] | 226.1 | [1] | 143.5 | [1], [5] | 626.2 | [2] | 0.519766 | [2] |
| 50% heptane, 50% isooctane | | | 371.9 | Calculated | 273.7 | Calculated | 174.2 | Calculated | 684.8 | Calculated | 1.07885 | Calculated |
| 90% heptane, 10% ethanol | | | 369.5 | Calculated | 271.4 | Calculated | 180.2 | Calculated | 690.7 | Calculated | | |
| 90% isooctane, 10% ethanol | | | 370.2 | Calculated | 278.5 | Calculated | 165.2 | Calculated | 699.8 | Calculated | | |
| 80% heptane, 20% isooctane | | | 371.7 | Calculated | 271.4 | Calculated | 179.2 | Calculated | 681.8 | Calculated | 1.00987 | Calculated |
| 63% heptane, 27% isooctane, 10% ethanol | | | 369.7 | Calculated | 273.5 | Calculated | 175.7 | Calculated | 693.4 | Calculated | | |
| 54% heptane, 36% isooctane, 10% ethanol | | | 369.8 | Calculated | 274.2 | Calculated | 174.2 | Calculated | 694.3 | Calculated | | |
| 60% heptane, 40% isooctane | | | 371.9 | Calculated | 272.9 | Calculated | 175.9 | Calculated | 683.8 | Calculated | 1.05586 | Calculated |
| 45% heptane, 45% isooctane, 10% ethanol | | | 369.9 | Calculated | 275.0 | Calculated | 172.7 | Calculated | 695.2 | Calculated | | |
| 45% heptane, 55% isooctane | | | 372.0 | Calculated | 274.1 | Calculated | 173.4 | Calculated | 685.3 | Calculated | 1.09034 | Calculated |
| 36% heptane, 54% isooctane, 10% ethanol | | | 369.9 | Calculated | 275.6 | Calculated | 171.2 | Calculated | 696.1 | Calculated | | |
| 27% heptane, 63% isooctane, 10% ethanol | | | 370.0 | Calculated | 276.4 | Calculated | 169.7 | Calculated | 697.0 | Calculated | | |
| 30% heptane, 70% isooctane | | | 372.1 | Calculated | 275.3 | Calculated | 170.9 | Calculated | 686.8 | Calculated | 1.12483 | Calculated |
| 18% heptane, 72% isooctane, 10% ethanol | | | 370.1 | Calculated | 277.1 | Calculated | 168.2 | Calculated | 698.0 | Calculated | | |
| 15% heptane, 85% isooctane | | | 372.2 | Calculated | 276.5 | Calculated | 168.4 | Calculated | 688.3 | Calculated | 1.15931 | Calculated |
| 9% heptane, 81% isooctane, 10% ethanol | | | 370.1 | Calculated | 277.8 | Calculated | 166.7 | Calculated | 698.9 | Calculated | | |
| 9.5% heptane, 85.5% isooctane, 5% ethanol | | | 371.2 | Calculated | 277.3 | Calculated | 167.1 | Calculated | 693.9 | Calculated | | |
| toluene | C7H8 | 108-88-3 | 383.9 | [1] | 277.6 | [1] | 178.2 | [1] | 862.3 | [2] | 1.18 | [2] |
| 70% Jet-A, 30% limonene | | | | | | | | | | | | |
| SPK | | | 501.1 | [8] | 317.1 | [8] | | | 762.0 | [8] | 3.8 | [8] |
| 50% Jet-A, 50% limonene | | | | | | | | | | | | |
| 50% Jet-A, 50% ATJ | | | | | | | | | | | | |
| pi e | C10H18 | 473-55-2 | 433.2 | [1] | 313.1 | [1] | 216.8 | [1] | | | 4.53 | [2] |
| 2,6-dimethyloctane | C10H22 | 2051-30-1 | | | | | | | 733.0 | [2] | | |
| HEFA | | | 542.5 | Measured | 314.1 | Measured | 226.2 | Measured | 761.2 | Measured | 5.571 | Measured |
| RJ4 | | | | | | | | | | | | |
| farnesane | C15H32 | 3891-98-3 | 524.1 | [9] | 381.1 | [9] | 195.2 | [9] | 773.0 | [9] | | |
| 1,4-dimethylcyclooctane | C10H20 | 33657-56-6 | | | 323.1 | [10] | | | 827.0 | [10] | 4.17 | [10] |
| p-menthane | C10H20 | 99-82-1 | 443.6 | [1] | | | 184.4 | [1] | | | | |
| ATJ | | | 536.1 | [11] | 323.1 | [11] | 183.2 | [11] | 761.0 | [11] | | |
| 90% Jet-A, 10% limonene | | | | | | | | | | | | |
| 50% Jet-A, 50% HEFA | | | 550.5 | Measured | 315.6 | Measured | 224.2 | Measured | 786.1 | Measured | 4.918 | Measured |
| 80% Jet-A, 20% limonene | | | | | | | | | | | | |
| methanol | CH4O | 67-56-1 | 337.7 | [1] | 284.0 | [1], [6] | 175.4 | [1], [5] | 796.0 | [2] | 1.36 | [2] |
| sabi e | C10H14 | | | | | | | | | | | |
| isopropyl | C3H8O | 67-63-0 | 355.7 | [1] | 285.0 | [1], [6] | 184.3 | [1], [5] | 789.2 | [2] | | |
| JETA | | | 558.1 | Measured | 318.1 | Measured | 231.2 | Measured | 810.8 | Measured | 4.502 | Measured |
| F-24 | | | | | | | 215.2 | Supplier | 803.2 | Supplier | 4.15 | Supplier |
| ethanol | C2H6O | 64-17-5 | 351.4 | [1] | 286.1 | [1], [6] | 159.1 | [1], [5] | 789.0 | [2] | 3.3892 | [2] |
| limonene | C10H16 | 138-86-3 | 450.9 | [1] | 323.1 | [1] | 178.2 | [1] | | | | |
| 90% Jet-A, 10% HEFA | | | 556.5 | Measured | 317.6 | Measured | 227.2 | Measured | 805.9 | Measured | 4.503 | Measured |
| 80% Jet-A, 20% HEFA | | | 555.0 | Measured | 317.1 | Measured | 229.2 | Measured | 801.0 | Measured | 4.629 | Measured |
| 70% Jet-A, 30% HEFA | | | 553.5 | Measured | 316.6 | Measured | 225.2 | Measured | 796.0 | Measured | 4.721 | Measured |

## S-4. Model Features

The figures below show all the features used in the property prediction models.

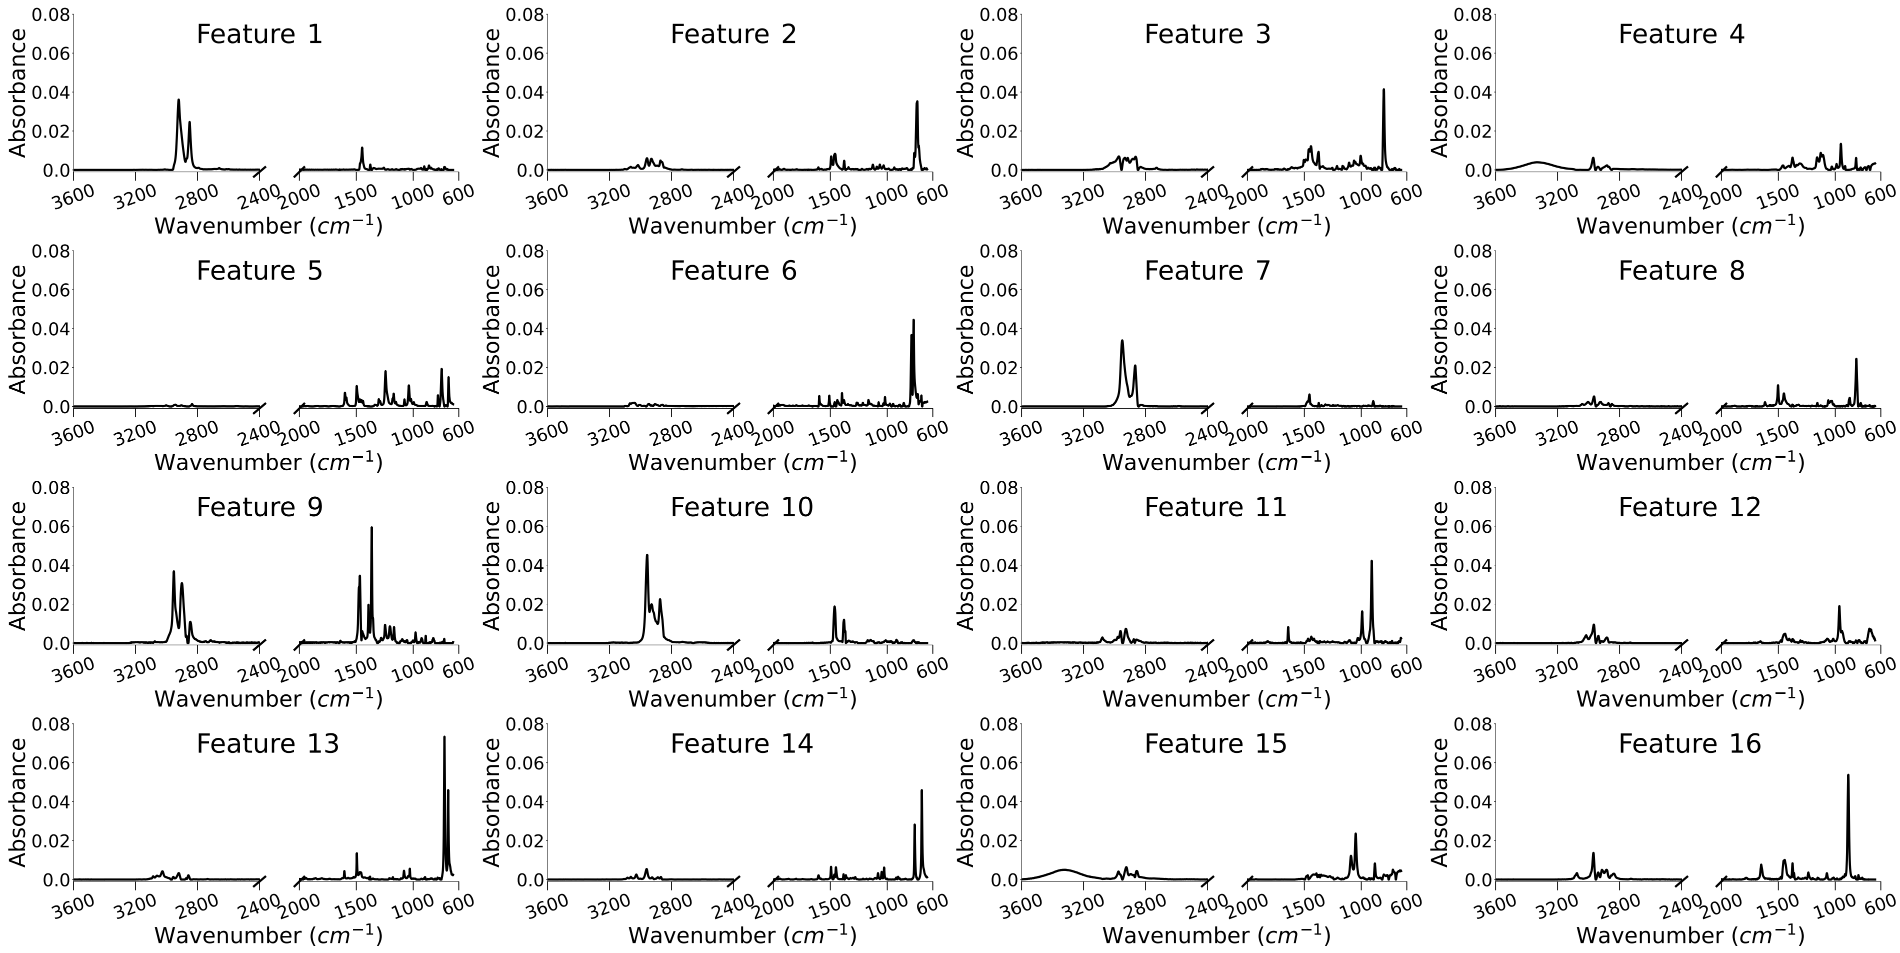


Figure S2: All features used in the final boiling point model

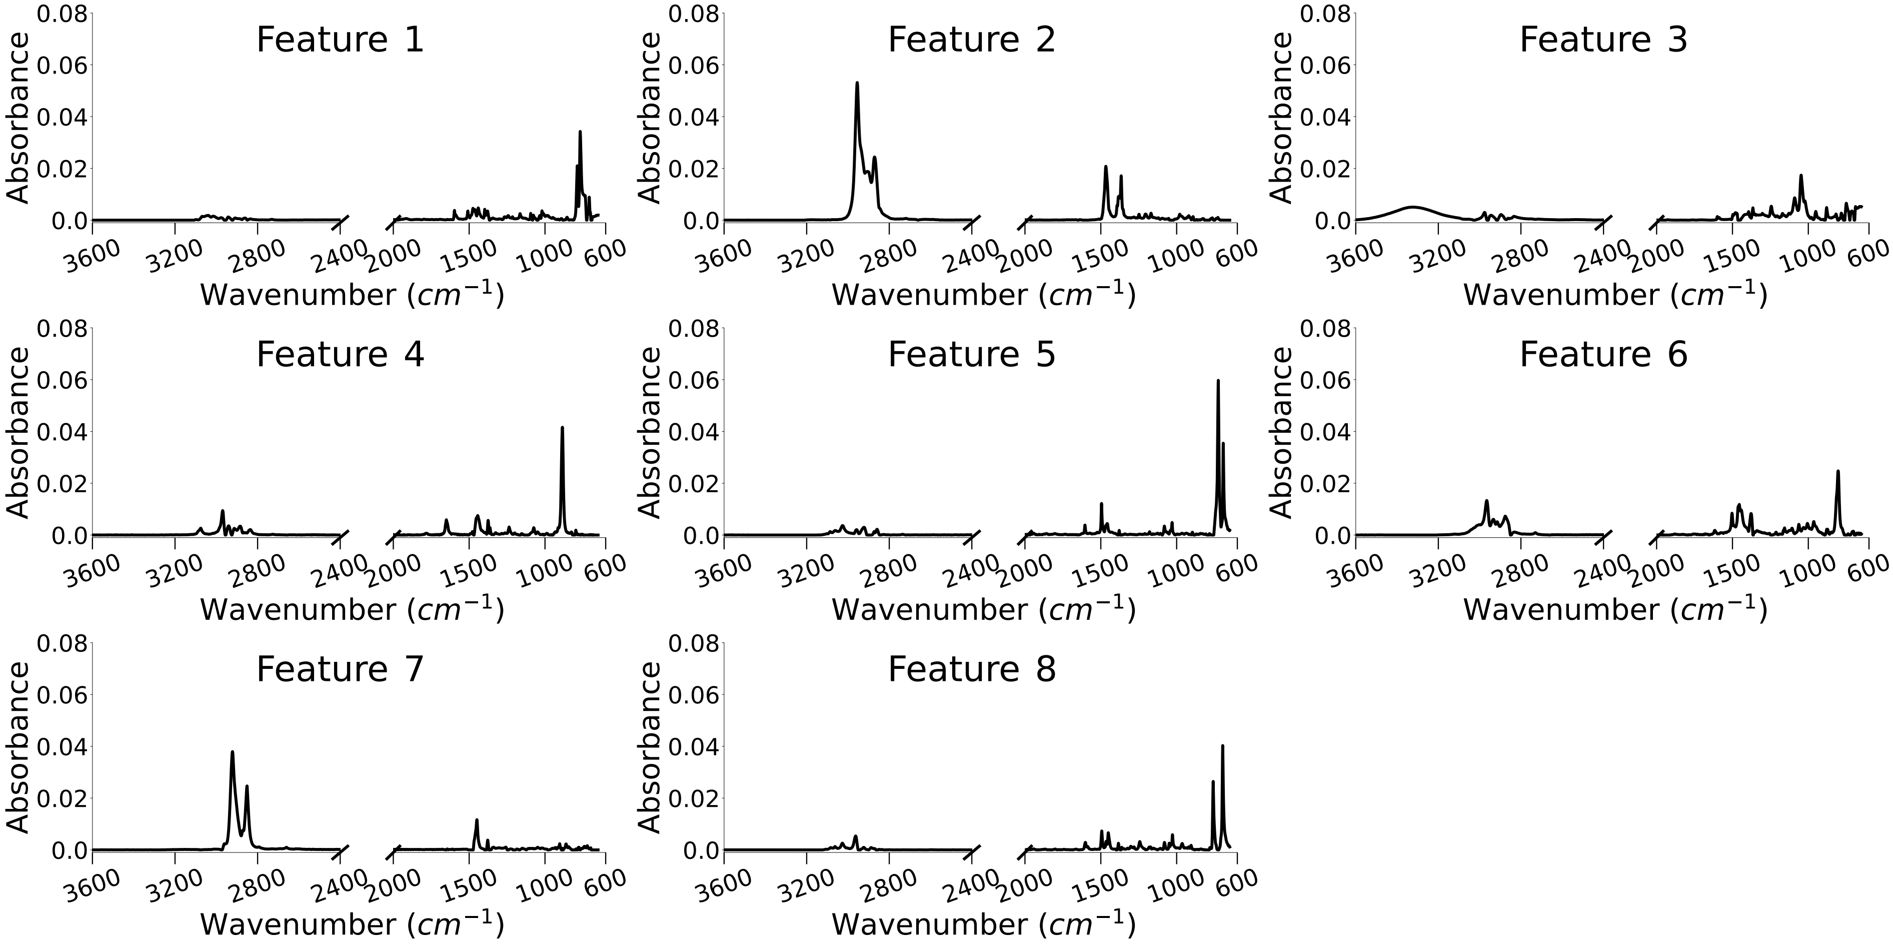


Figure S3: All features used in the flash point model

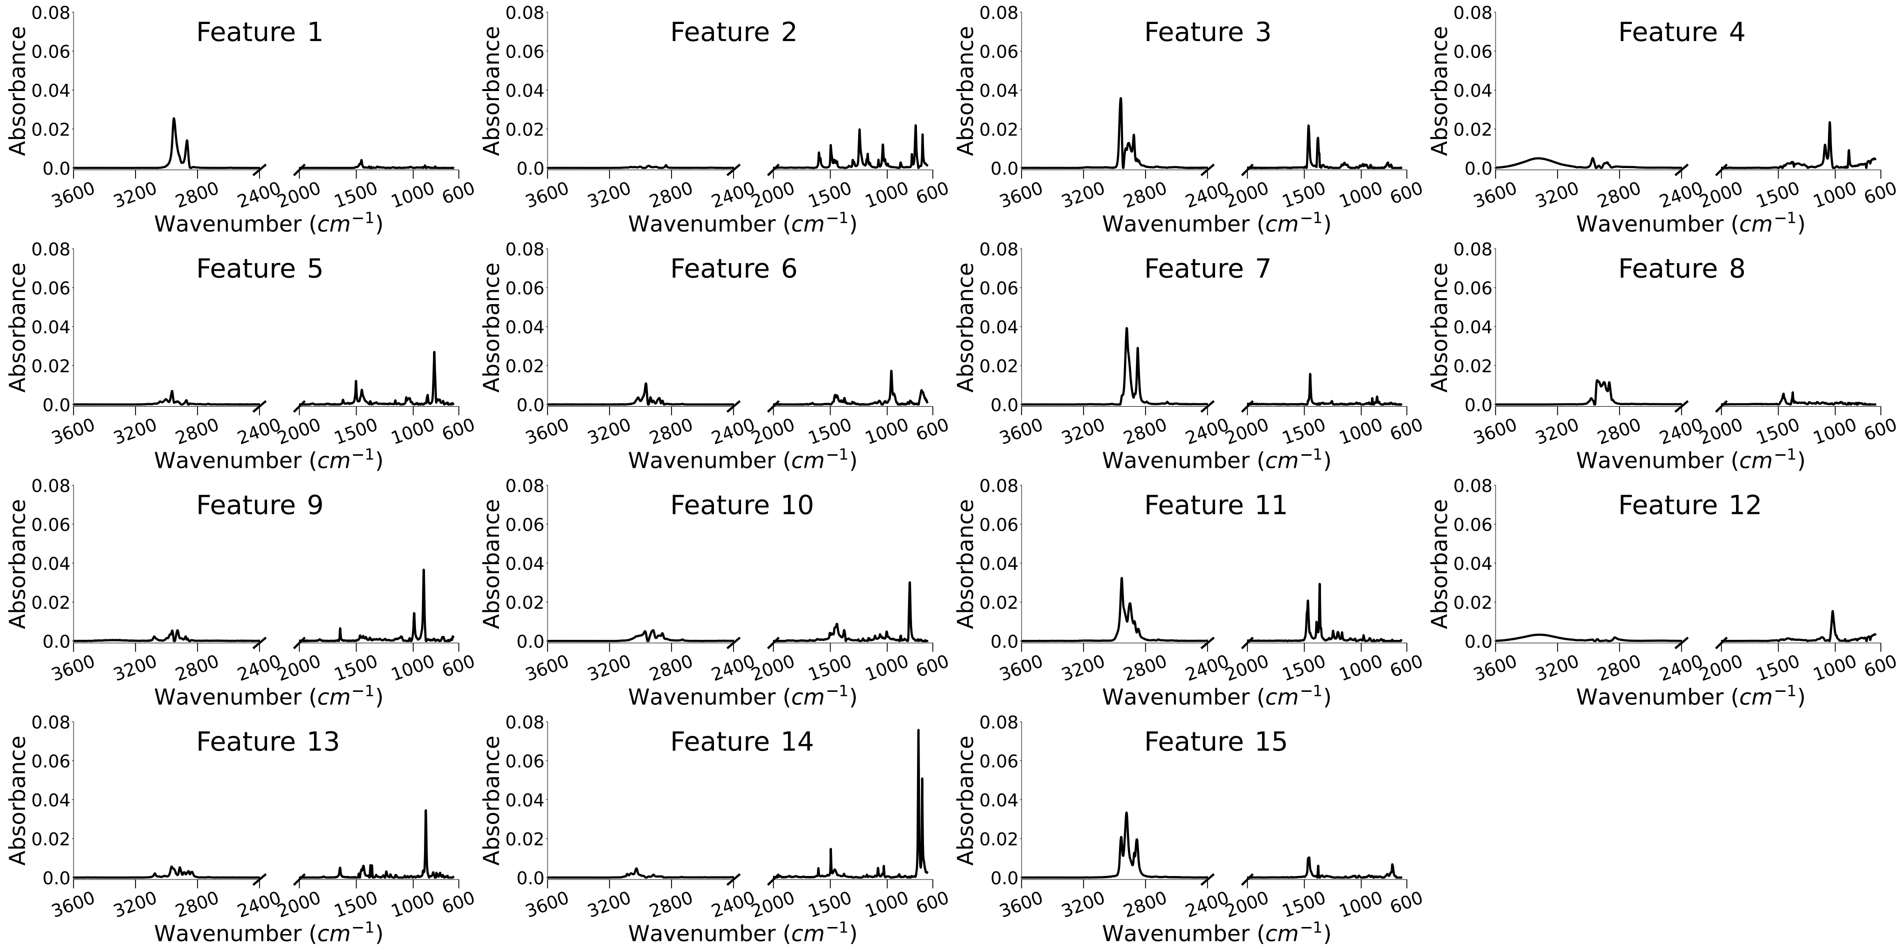


Figure S4: All features used in the freezing point model

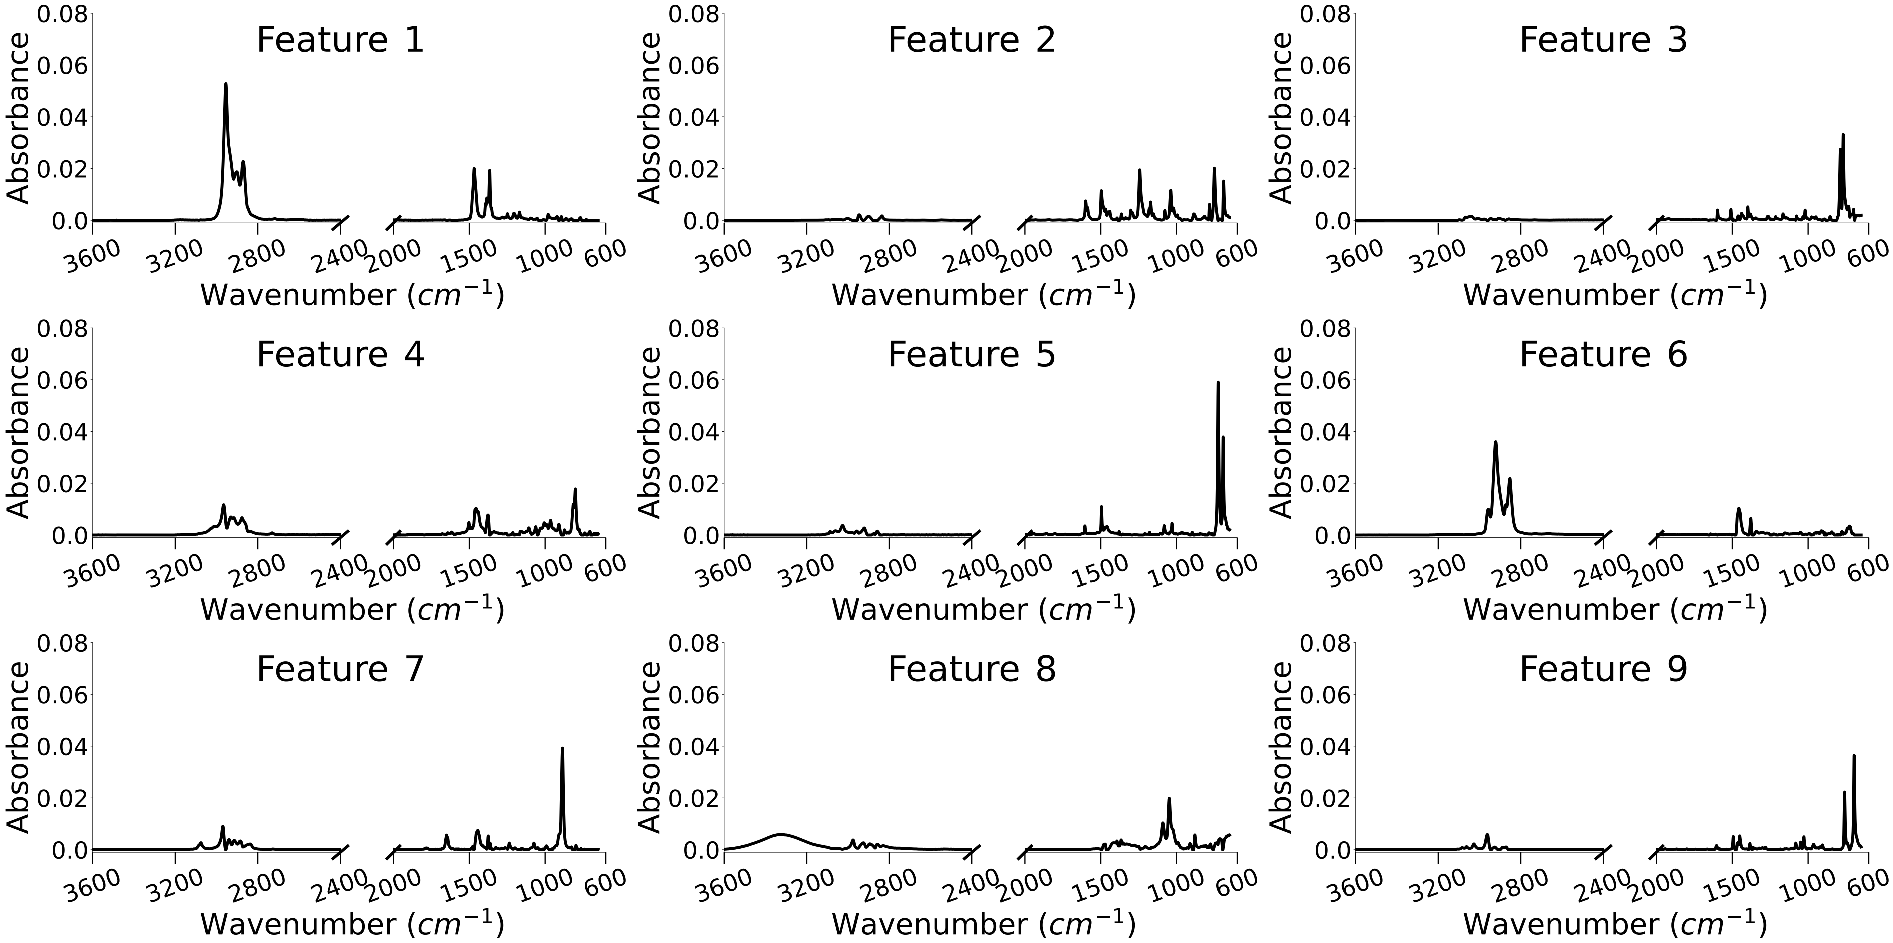


Figure S5: All features used in the density model

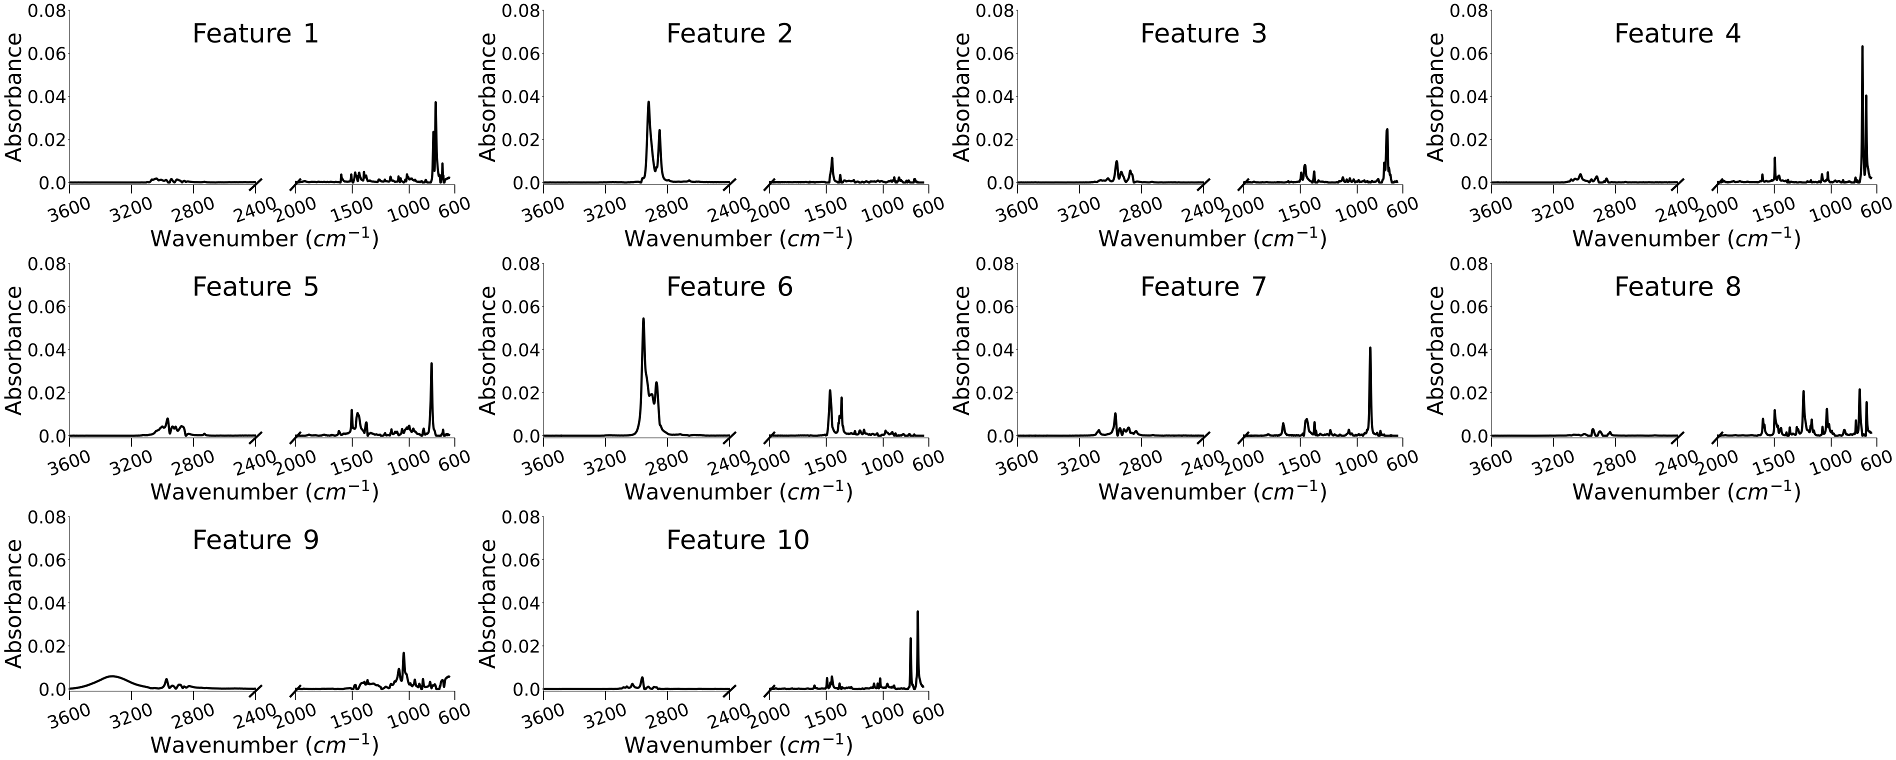


Figure S6: All features used in the kinematic viscosity model

**References**

[1] S. Kim, J. Chen, T. Cheng, A. Gindulyte, J. He, S. He, Q. Li, B. A. Shoemaker, P. A. Thiessen, B. Yu, L. Zaslavsky, J. Zhang, E. E. Bolton, PubChem 2019 update: improved access to chemical data, Nucleic Acids Research 47 (D1) (2018) D1102–D1109. doi:10.1093/nar/gky1033.

[2] Springer materials.
URL `https://materials.springer.com/`

[3] Chemspider.
URL `https://www.chemspider.com/`

[4] N. R. E. Laboratory, Co-optimization of fuels & engines: Fuel properties database.
URL `https://www.nrel.gov/transportation/fuels-properties-database/`

[5] J.-C. Bradley, A. Williams, A. Lang, Jean-Claude Bradley Open Melting Point Dataset (May 2014). doi:10.6084/m9.figshare.1031637.v2.

[6] D. A. Saldana, L. Starck, P. Mougin, B. Rousseau, L. Pidol, N. Jeuland, B. Creton, Flash point and cetane number predictions for fuel compounds using quantitative structure property relationship (QSPR) methods, Energy & Fuels 25 (9) (2011) 3900–3908. doi:10.1021/ef200795j.

[7] C. L. Yaws, Chapter 1 - physical properties – organic compounds, in: C. L. Yaws (Ed.), The Yaws Handbook of Physical Properties for Hydrocarbons and Chemicals (Second Edition), second edition Edition, Gulf Professional Publishing, Boston, 2015, pp. 1–683. doi:10.1016/B978-0-12-800834-8.00001-3.

[8] J. Yang, Z. Xin, Q. S. He, K. Corscadden, H. Niu, An overview on performance characteristics of bio-jet fuels, Fuel 237 (2019) 916–936. doi:10.1016/j.fuel.2018.10.079.

[9] Olivier Rolland, Fernando Garcia, Evaluation of Synthesized Iso-Paraffins produced from Hydroprocessed Fermented Sugars (SIP Fuels), Final report, TOTAL New Energies, Amyris, Inc., and United States Air Force Research Laboratory (Feb. 2014).

[10] K. Rosenkoetter, C. Kennedy, P. Chirik, B. Harvey, [4+4]-cycloaddition of isoprene for the production of high-performance bio-based jet fuel, Green Chemistry 21 (09 2019). doi:10.1039/C9GC02404B.

[11] J. Edwards, Reference jet fuels for combustion testing, 2017. doi:10.2514/6.2017-0146.
